# Supplementary material for: NexusSplats: Efficient 3D Gaussian Splatting in the Wild
Source: arXiv:2411.14514 source file (2025-03-09)
Supplement: Supplementary file 1 [file 6_suppl.tex]

\clearpage
\setcounter{page}{1}
\maketitlesupplementary
\appendix

%-------------------------------------------------------------------------
\section*{Overview}
%-------------------------------------------------------------------------
\section*{Reproducibility}
%-------------------------------------------------------------------------
\section*{Video Demo}
%-------------------------------------------------------------------------
\section{Implementation Details}
\label{sec:implementation}
%-------------------------------------------------------------------------
\section{Comparisons on NeRF On-the-go}
\label{sec:full results}
%-------------------------------------------------------------------------
\section{Further Visualizations}
\label{sec:visualization}
%-------------------------------------------------------------------------
\section{Discussions and Limitations}
